# Supplementary material for: TokenMixup: Efficient Attention-guided Token-level Data Augmentation for Transformers
Source: arXiv:2210.07562 source file (2022-10-14)
Supplement: Supplementary file 2 [file appendix_algos.tex]

\begin{algorithm}[ht!]
\caption{TokenMixup -- Full Version}
\label{alg:htm_v2_full}
\textbf{Input:} $X \in \rm I\!R^{b \times n \times d}$, $Y \in \rm I\!R^{b \times c}$, $\tau$, $\rho$\\
\textbf{Output:} $Z \in \rm I\!R^{b \times n \times d}$, $Y, \hat{Y} \in \rm I\!R^{b \times c}$
\begin{algorithmic}[1]
    % \State $A \gets \textrm{forward self attention with stop-gradient to retrieve attention map}$
    \State $\hat{Y} \gets \textrm{ScoreNet}(X)$
    \State $U \gets \textrm{CrossEntropy(Softmax}(\hat{Y}), Y)$ \hfill $\triangleright$ Eq. (1)
    \State $A \gets \textrm{apply $\ell$-step attention rollout}$ \hfill $\triangleright$ Eq. (2)
    \State $S_t \gets \frac{1}{n}\sum_{i=1}^n  A_{i,t} \:\:\:\:\:\: \textrm{s.t.} \:\: t=1,2,\ldots,n$ \hfill $\triangleright$ Eq. (3)
    \State idx $\gets $ sample indices where $U < \tau$
    \State $b' \gets \textrm{number of items in idx}$
    \State $\tilde{X}, \tilde{Y}, \tilde{S} \gets X[\textrm{idx}], Y[\textrm{idx}], S[\textrm{idx}]$
    \State $C_{ij} \gets \sum_{t} \textrm{max}({S}_t^{(j)} - \tilde{S}_t^{(i)} - \rho,\: 0) \:\:\:\:$ s.t. $i = 1, 2, \ldots, b'$ and $j = 1, 2, \ldots, b$ \hfill $\triangleright$ Eq. (6)
    \State $\sigma(m) \gets \textrm{HungarianMatching}(C_{ij})\:\:\:\:$ s.t. $m = 1, 2, \ldots, b'$  and $\sigma (m) \in \{1, 2, \ldots, b\}$ \hfill $\triangleright$ Eq. (7)
    \For{sample index $m = 1, 2, \ldots, b'$}
    \State $M_t \gets 0 \;\; \textrm{ if } S_t^{(\sigma(m))} - \tilde{S}_t^{(m)} > \rho \;\; \textrm{ else } 1 \:\:\:\:$ s.t. $t = 1, 2, \ldots, n$ \hfill $\triangleright$ Eq. (9)
    \State $\tilde{X}^{(m)} \gets M \odot \tilde{X}^{(m)} + (1-M) \odot X^{(\sigma(m))}$ \:\:\:\: s.t. $M = [M_t]_{t=1}^n$  \hfill $\triangleright$ Eq. (10)
    \State $\tilde{Y}^{(m)} \gets  \frac{\sum_t M_t \cdot \tilde{S}_t^{(m)}}{\sum_t M_t \cdot \tilde{S}_t^{(m)} + (1-M_t) \cdot S_t^{(\sigma(m))}} \tilde{Y}^{(m)} + \frac{\sum_t (1-M_t) \cdot S_t^{(\sigma(m))}}{\sum_t M_t \cdot \tilde{S}_t^{(m)} + (1-M_t) \cdot S_t^{(\sigma(m))}} Y^{(\sigma(m))}$ \hfill $\triangleright$ Eq. (11)
    \EndFor
    \State $X \gets X[\neg \textrm{ idx}] \cup \tilde{X} \:\:\:\:$ s.t. $\tilde{X} = \{\tilde{X}^{(m)}\}_{m=1}^{b'}$
    \State $Y \gets Y[\neg \textrm{ idx}] \cup \tilde{Y} \:\:\:\:$ s.t. $\tilde{Y} = \{\tilde{Y}^{(m)}\}_{m=1}^{b'}$
    \State $Z \gets \textrm{MultiHeadSelfAttention}(X)$
    \State \textbf{return } $Z$, $Y$, $\hat{Y}$
\end{algorithmic}
\end{algorithm}

\begin{algorithm}[ht!]
\caption{Vertical TokenMixup}
\label{alg:vtm}
\textbf{Input:} $X \in \rm I\!R^{b \times n \times d}$, $Y \in \rm I\!R^{b \times c}$, $\kappa$ \\
\textbf{Output:} $Z \in \rm I\!R^{b \times n \times d}$
\begin{algorithmic}[1]
    \State $L \gets $ previous layer indices
    \For{layer index $l \in L$}
    \State $X^{(l)} \gets$ token input for layer $l$
    \State $A^{(l)} \gets \textrm{apply $\ell$-step attention rollout}$ \hfill $\triangleright$ Eq. (2)
    \State $S_t \gets \frac{1}{n}\sum_{i=1}^n  A_{t,i}^{(l)} \:\:\:\:\:\: \textrm{s.t.} \:\: t=1,2,\ldots,n$ \hfill $\triangleright$ Eq. (3)
    \State $X^{(l)} \gets $ select top $\kappa$ tokens w.r.t \: $ S_t$
    \EndFor
    \State $X' \gets \underset{l \in L'}{\bigcup} X^{(l)} \:\:\:\:\:\: \textrm{s.t. } L' = \{l_0\} \cup L \textrm{ and } l_0 =$ current layer index
    \State $Z \gets \textrm{MultiHeadCrossAttention}(\textrm{query}=X, \textrm{key}=X', \textrm{value}=X')$ \hfill $\triangleright$ Eq. (13)
    \State \textbf{return } $Z$
\end{algorithmic}
\end{algorithm}
